# Supplementary material for: Confidence-aware Fine-tuning of Sequential Recommendation Systems via Conformal Prediction
Source: arXiv:2402.08976 source file (2025-02-20)
Supplement: Supplementary file 1 [file Appendix.tex]

%%
%% If your work has an appendix, this is the place to put it.
\appendix

\section{Method Details}

\subsection{Split Conformal Prediction}
\label{Appdendix: Split CP}
A classical version of Split Conformal Prediction is detailed with Algorithm \ref{algo1}.

\begin{algorithm}
\caption{Split Conformal Prediction}
\label{algo1}
\begin{algorithmic}[1]
    \Require  Training Data $D$, Calibration set size $n$,
            Calibration set of size $n$,
            Test point $X_{n+1} = x$,
            Prediction model $\hat{f}$,
            Score function $s(x,y)$,
            Desired error rate $\alpha$.
    
    \State {Randomly hold out $n$ samples as calibration set $D_c$, and the remaining samples is represented as training set $D_{tr}$.}
    \State{Fit model $\hat{f}$ on training set $D_{tr}$.}
    \State{Predict the label of samples in calibration set $D_c$ and test sample with $\hat{f}$.}
    \State{Compute the scores of $D_c$ using $s(x,y)$, get score set $S = \{s(X_i,Y_i)\}^{n}_{i=1}$.}
    \State{Compute quantile value $\hat{q}_{1-\alpha}$ of score set $S$ at $\lceil(1-\alpha)(1+\frac{1}{n}) \rceil$ level.}
    \State{Construct pr ediction set for test sample $\hat{C}(X_i) = \{ y: s(X_i,y) \leq \hat{q}_{1-\alpha}\}$.}
    
    \Ensure Prediction set $\hat{C}(X_{n+1})$.
\end{algorithmic}
\end{algorithm}
